# Supplementary material for: Technical Report of NICE Challenge at CVPR 2024: Caption Re-ranking Evaluation Using Ensembled CLIP and Consensus Scores
Source: arXiv:2405.01028 source file (2024-06-13)
Supplement: Supplementary file 1 [file X_suppl.tex]

\clearpage % ensures that all floats are processed

\setcounter{page}{1} % reset page counter if necessary
\maketitlesupplementary
% \onecolumn

% Assuming "why an dae" is a placeholder text. Replace with actual section title if needed.
\section*{A. Results of all Metrics} % Use the '*' to remove the section number

% First subsection and table
\subsection*{A1. Effects of Caption Filtering} % Use the '*' to remove the subsection number

\begin{table}[!ht] % 'htbp' gives LaTeX more flexibility
    \centering
    \resizebox{\textwidth}{!}{ % Resize to text width for better fit
    \begin{tabular}{@{}lcccccccc@{}}
      \toprule
      Method & CIDEr & SPICE & METEOR & ROUGE-L & BLEU$_{\text{AVG}}$\\
      \midrule
      (b) Consensus Score & \textbf{202.89} & \textbf{31.21} & \textbf{35.79} & \textbf{68.20} & \textbf{67.07} \\
      (e) Consensus Score (w/o Caption Filtering) & 192.98 & 30.10 & 34.41 & 65.89 & 64.75 \\
      \bottomrule
    \end{tabular}
    }
    \caption{\textbf{Ablations of Caption Filtering.} \textbf{(e)} has the same settings as \textbf{(b)} with the exception of using a caption filter.}
    \label{tab:table4}
\end{table}

% Second subsection and table
\subsection*{A2. Effects of the Short Caption Selection} % Use the '*' to remove the subsection number
\begin{table}[!ht] % 'htbp' gives LaTeX more flexibility
    \centering
    \resizebox{\textwidth}{!}{ % Resize to text width for better fit
    \begin{tabular}{@{}lcccccccc@{}}
      \toprule
      Method & CIDEr & SPICE & METEOR & ROUGE-L & BLEU$_{\text{AVG}}$\\
      \midrule
      (d) Ensembled CLIP Score + 3.52*Consensus Score & 218.47 & \textbf{33.46} & \textbf{37.98} & 70.13 & 67.58 \\
      (f) \hspace{8.7em} + Short Capation Selection & \textbf{220.53} & 33.01 & 37.68 & \textbf{70.31} & \textbf{69.20} \\
      \bottomrule
    \end{tabular}
    }
    \caption{\textbf{Ablations of Short Caption Selection.} \textbf{(f)} has the same settings as \textbf{(d)} with the addition of Short Caption Selection. We set the threshold $\mathbf{\theta}$ to 0.39.} 
    \label{tab:table5}
\end{table}
