# Supplementary material for: Technical Report of NICE Challenge at CVPR 2024: Caption Re-ranking Evaluation Using Ensembled CLIP and Consensus Scores
Source: arXiv:2405.01028 source file (2024-06-13)
Supplement: Supplementary file 2 [file appendix_table1.tex]

\centering
  \begin{tabular}{@{}lcccccccc@{}}
    \toprule
    Method & CIDEr & SPICE & METEOR & ROUGE-L & BLEU_{\text{AVG}}\\
    \midrule
    \midrule
    (b) Consensus Score & \textbf{202.89} & \textbf{31.21} & \textbf{35.79} & \textbf{68.20} & \textbf{67.07} \\
    (e) Consensus Score (w/o Caption Filtering) & 192.98 & 30.10 & 34.41 & 65.89 & 64.75 \\
    \bottomrule
\end{tabular}
