# Supplementary material for: Technical Report of NICE Challenge at CVPR 2024: Caption Re-ranking Evaluation Using Ensembled CLIP and Consensus Scores
Source: arXiv:2405.01028 source file (2024-06-13)
Supplement: Supplementary file 3 [file appendix_table2.tex]

\centering
\begin{tabular}{@{}lcccccccc@{}}
  \toprule
  Method & CIDEr & SPICE & METEOR & ROUGE-L & BLEU_{\text{AVG}}\\
  \midrule
  \midrule
  (d) Ensembled CLIP Score + 3.52*Consensus Score & 218.47 & \textbf{33.46} & \textbf{37.98} & 70.13 & 67.58 \\
  (f) \hspace{10.3em} { + Short Cap Selection} & \textbf{220.53} & 33.01 & 37.68 & \textbf{70.31} & \textbf{69.20} \\
  \bottomrule
\end{tabular}
